# Supplementary material for: Harmonic Chain Barcode and Stability
Source: arXiv:2409.06093 source file (2024-09-09)
Supplement: Supplementary file 1 [file sec-appendix.tex]

\section{Deriving Harmonic Chain Barcodes From Persistence Barcodes}
\label{sec:unstable-harmonic-barcode}

\subsection{Harmonic barcodes out of persistence barcode}\label{sec:harmonicdiagram}

We now give a formal definition of the {\hcd}. We first choose a basis for persistent homology. Each scheme for choosing a basis defines a type of {\hcd}. 
Consider the persistence module of homology groups $H(F)$.
Recall that $H(F)$ can be written uniquely as a summation of interval modules,
\begin{equation}
H(F) \cong \bigoplus_{j} I(b_j,d_j).
\end{equation}

Let $B = \{[b_j,d_j)\}$ be the collection of intervals, where $b_i,d_i \in \Rspace \cup \{+\infty\}$. We fix an isomorphism $\phi = \{\phi_t\}$ realizing the above relation, which amounts to choosing a basis element for each interval. More formally, let $\phi_t: B \rightarrow H(K_t)$ be functions such that,
\begin{enumerate}
\item $\phi_t$ maps intervals $[b_i,d_i)$ injectively to a collection of basis elements in $H(K_t)$ for $b_i \leq  t < d_i$, and other intervals to $0$;
\item The non-zero images of the same interval under different $\phi_t$, are mapped to each other by the homomorphisms $f^*_i$.
\end{enumerate}

A choice of basis satisfying these two conditions is, for instance, provided by the persistence reduction algorithm~\cite{edelsbrunner2002topological,zomorodian2005topology} used to compute the ordinary persistence barcode.

Next, we define a new persistence module $\Gamma = \Gamma(\phi)$ as follows. For all $r\in \Rspace$, we set $\Gamma_r = H(F_r)$. For any $s<t$, we define new homomorphisms $g_s^t: H(K_{s}) \rightarrow H (K_{t})$, by defining their value on the basis elements $\phi_t(B)$. Let $h \in H(K_{t})$ be a non-zero homology class in the image of $\phi_t$. There is a unique cycle $z \in h$ which is also a cocycle.  We set $g_s^t(h) = f_{s*}^t(h)$ if $z$ is a cocycle in $K_{t}$, and, $g_s^t(h) = 0$ otherwise. We call $\Gamma$ the \emph{harmonic filtration subordinate to $\phi$}. This is a persistence module. 

It follows from the decomposition theorem for persistence modules~\cite{crawley2015decomposition} that the filtration $\Gamma$ can be written as a linear combination of basis interval modules. Each interval module has a birth and a death time. We call the collection of these intervals the \emph{harmonic persistence barcode subordinate to $\phi$}, and we call 
the corresponding barcode, the \emph{\hcd} \emph{subordinate to $\phi$}. 

Observe that each harmonic interval, by definition of the $g_s^t$, corresponds to a unique harmonic cycle. The harmonic persistence barcode therefore tracks features which have a very well-defined and unique geometric entity associated with them. 



\subsection{Example}

Figure~\ref{fig:harmonicexample} presents an example where we have computed the harmonic persistent barcode starting by the cycles for the bars computed by the standard reduction algorithm. 
We use the time stamps as the names of the simplices. Also we give simplices the standard orientation determined by the ordering of the vertices given by the insertion time. The procedure we describe gives an algorithm of running time $O(n^4)$ where $n$ is the number of simplices.


Let $B_1=[9,t_4]$ be the longest bar in the persistence barcode, it is represented by the cycle $z_1 = 7+8-9$. Let $B_2 = [11, t_3]$ be the next longest bar, $z_2 = -11 +10 +9$.  Let $B_3 = [13,t_2]$ be the next bar, it is represented by $z_3=13-12+9$. Finally, let $B_4 = [15,t_1]$ be the last bar, it is represented by $z_4=15-14+9$.

To obtain harmonic bars we sweep from left to write. At time $t_1$, all of the basis cycles $z_i$ get a coboundary. From these, the homology class of $z_4$ becomes trivial, and others are still non-trivial. For instance, if we take $z_1$, its homology class is still non-trivial. We can find a new harmonic cycle in its class by finding $x$ such that $\delta(z_1 + \partial x) =0$ at time $t_1$. This implies $-t_1 = \delta(z_1) = - \delta \partial x$. Since $\delta \partial t_1 = 3 t_1$, we can set $x = 1/3 t_1$, and the new harmonic chain is $z^1_1 = z_1 + 1/3 \partial (t_1)$. We get similarly $z^1_2 = z_2 - 1/3 \partial (t_1)$ and $z^1_3 = z_3 - 1/3 \partial (t_1)$. At time $t_2$, $z_3$ and hence $z^1_3$ die. Cycle, $z^1_1$ gets a coboundary $- t_2$ and $\delta t_1$ gets a coboundary $t_2$ hence $\delta_{t_2} (z^1_1) = -2/3 t_2$. A new harmonic cycle is $z_1^2 = z_1 + 1/4(\partial t_1 + \partial t_2)$. Similarly, $z^2_2 = z_2 - 1/4(\partial t_1 + \partial t_2)$. At time $t_3$, the cycle $z_2$ and its harmonic homologous cycles die. $z_1^2$ also becomes non-harmonic and will be replaced by another harmonic cycle that will die at $t_4$. 

We note that although each harmonic chain becomes non-harmonic after insertion of a simplex in this example, this is not a general phenomenon. The harmonic bars can be long.


\begin{figure}
    \centering
    \includegraphics[scale = 0.75]{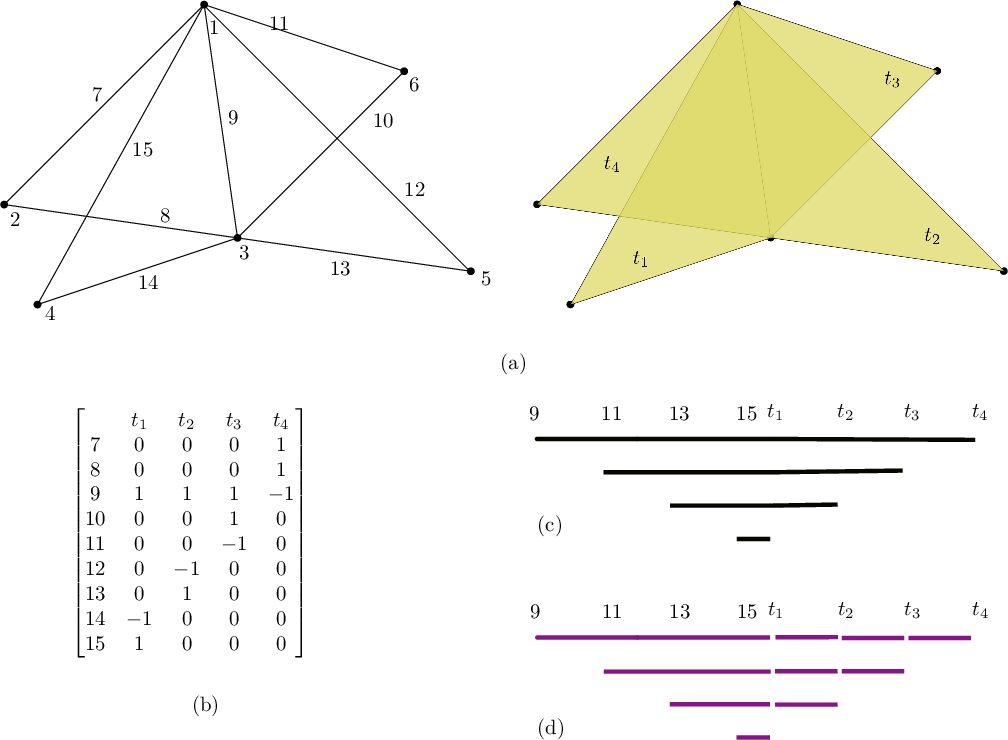} 
    \caption{(a) A filtration of a simplicial complex, the time that a simplex is inserted is written next to the simplex. For the four triangles we have times $t_1 < t_2 < t_3 < t_4$. We also use these time stamps as the name of the simplex. (b) Part of the boundary matrix of the complex which is relevant to 1-dimensional homology. The boundary matrix is already reduced, therefore, the generators of persistent homology computed by the standard reduction algorithm are given by columns of the matrix. (c) The ordinary persistence barcode. (d) The harmonic barcode based on the cycles computed by the standard reduction algorithm.}
    \label{fig:harmonicexample}
\end{figure}

\subsection{Computation}

In this section, we prove that the procedure of Section~\ref{ssec:computation} for computing the harmonic chain barcode is correct. We start by assuming that in the filtration $F$ we add a single simplex at a time.
Under this assumption, we compute the canonical harmonic diagram by sweeping time from $-\infty$ to $\infty$. At any time $t$, we maintain a set of cycles $R(t)$ satisfying the invariant that,%For these purposes, we obtain the same set of bars by a different process where we sweep the parameter $t$ from $-\infty$ to $\infty$, and we maintain a set of cycles $R(t)$ satisfying the invariant that, at any time $t$,

\begin{itemize}
    \item the set $R(t)$ contains cycles realizing a lex.-maximal independent span-length sequence for $Z(K_t) \subset Z(K)$.
\end{itemize}


%That is to say, $R(t)$ contains cycles from $K_t$, and those representatives are still harmonic at $t$. $R(t)$ is then
%a basis for $\har_d(K_t)$. The set of spans defined by the cycles in the union of $R(t)$ can be taken as a second definition 
%of a canonical harmonic diagram.

The following Lemma describes the change from $R(t_i)$ to $R(t_{i+1})$.


\begin{lemma}
\label{lemma:greedy}

    Assume that the harmonic representatives $R(t_{i})$ satisfy the invariant at time $t_i$. Then, at time $t_{i+1}$, if the dimension of the harmonic chains increases, to obtain $R(t_{i+1})$ satisfying the invariant, it is enough to add to $R(t_{i})$ the lex.-maximal set of independent spans born at $t_i$.
    
\end{lemma}


\begin{proof}
    Let $\sigma$ be the simplex inserted at time $t_{i+1}$. If $\sigma$ is not $d$ or $d+1$ dimensional then the set of $d$-cycles and harmonic $d$-cycles do not change. We then can set $R(t_{i+1})=R(t_{i})$.

    Suppose $\sigma$ is $d$-dimensional. Then it might create new harmonic cycles. If this does not happen we can set $R(t_{i+1})=R(t_{i})$. Note that a new harmonic cycle is created if and only if a new $d$-homology class is born. In this case, the dimension of harmonic cycles increases. Note that $\har (K_{t_{i}}) \subset \har (K_{t_{i+1}})$ is a subspace of codimension 1.
    
    Let $N$ be the maximum death time of all harmonic cycles generated at time $t_{i+1}$. Note that $N-t_{i+1}$ is the maximum span length of these cycles and their span is determined by their death time. Let $\zeta \in \har (K_{t_{i+1}})$ be a cycle that realizes the span $[t_{i+1},N]$. Set $R' = R(t_i) \cup \{ \zeta \}$. We claim that $R'$ satisfies the invariant at time $t_{i+1}$. %It is evident that $R'$ is a basis of $\har (K_{t_{i+1}})$. 

    To prove the claim we consider how the maximum span-length sequence of $Z(K_{t_{i+1}})$, denoted, $\rho_1 \geq \rho_2 \geq \cdots $ is constructed. Recall that we first take a cycle with maximum span length. If this cycle is in $Z(K_{t_{i}})$ then this span length will appear as span interval with maximum length in $R(t_i) \subset R'$ by the induction hypothesis. This will be again true for the second number, etc. Let $\rho_j$ be the first appearance of a number that is not in the maximum span-length sequence for $Z(K_{t_{i}})$ (note that it can be that $\rho_j = \rho_{j-1}$, in this case $\rho_j$ is one more repetition of the same number). A realizing cycle is in $Z(K_{t_{i+1}}) - Z(K_{t_{i}})$ and it has to have the maximum span length in this set. Therefore, $\rho_j = N-t_{i+1}$ and $\zeta$ realizes this span-length. Now we claim that the rest of the cycles in a sequence realizing the maximum span-length sequence for $Z(K_{t_{i+1}})$ must come from $Z(K_{t_{i}})$ and hence their span-lengths must appear among spans of $R(t_i) \subset R'$.

    To prove the claim let's assume for the sake of contradiction that a second cycle appearing in order of span-lengths $\zeta' \in Z(K_{t_{i+1}}) - Z(K_{t_{i}})$ has a span-length in the sequence, and $|span(\zeta')|\leq |span(\zeta)|$. $\zeta'$ must have a non-zero coefficient for $\sigma$ say $\beta$. Let $\alpha \neq 0$ be the coefficient of $\sigma$ in $\zeta$. We can form the cycle $\chi = \alpha/ \beta \zeta' - \zeta \in Z(K_{t_{i}})$. When $\chi$ becomes non-harmonic, i.e., at the first $t$ such that $\delta_t(\chi)\neq 0$, at least one of $\zeta'$ and $\zeta$ must also become non-harmonic. Since the death time of $\zeta$ is equal or larger than $\zeta'$, the death time of $\chi$ is at least that of $\zeta'$. Since $\chi$ already exists at time $t_{i}$ it must be that $|span(\chi)| > |span(\zeta')|$. This contradicts the selection of $\zeta'$ as it is in a space generated by cycles of larger span-length $\zeta$ and $\chi$. This finishes the argument.

    If $\sigma$ is $d+1$-dimensional, the set of $d$-cycles $Z(K_t)$ does not change and we can set $R(t_{i+1}) = R({t_i})$.

    
    
\end{proof}


Now we consider an arbitrary filtration $F$. Let $\Sigma_i$ be the set of simplices inserted at time $i$. We can simulate $F$ using a filtration which inserts $\Sigma$ one simplex at a time $t_{i,j}=t_{i,j'}$. In other words, we apply Lemma~\ref{lemma:greedy} one simplex at a time. We need however consider all the possible orderings for insertions. For any fixed ordering, the above lemma applies. We need to take the ordering which leads eventually to the lex. maximal sequence of spans added at time $t_{i+1}$. We can obtain this sequence by computing the new harmonic chain space $A = \har{K_{t_{i+1}}} - \har{K_{t_i}}$. All these chains are born at $t_{i+1}$. We need to choose first the longest such span, then the next independent largest span, and so on. Since the span-lengths in $A$ are determined by death times, this is what the procedure of Section~\ref{ssec:computation} computes. 




\begin{comment}
\begin{proof}

   

    Let $\Sigma$ be the set of simplices inserted at time $t_{i+1}$. We show the changes that happen to $d$-dimensional bars and write $R(t_i)$ for these bars.
    
    If $\Sigma$ does not contain $d$ or $d+1$ dimensional simplices then the set of $d$-cycles and harmonic $d$-cycles do not change. We then can set $R(t_{i+1})=R(t_{i})$.

    Suppose $\Sigma_d \subset \Sigma$ is the collection of $d$-dimensional simplices. Then it might create new harmonic cycles. If this does not happen we can set $R(t_{i+1})=R(t_{i})$. Note that a new harmonic cycle is created if and only if a new $d$-homology class is born. In this case, the dimension of harmonic cycles increases. 

    Let $(z_i)=z_1, z_2, \ldots$ be a sequence of independent harmonic chains realizing the lex.-maximal independent span-length sequence for $Z(K_{t_{i+1}})$ and $(y_i)=y_1, y_2, \ldots$ be such a sequence for $Z(K_{t_i})$. We claim that we can choose the sequence $(z_i)$ such all cycles which do not belong to $(y_i)$ are born at $t_{i+1}$. For this purpose, we choose $(z_i)$ such that it retains the maximum number of $y_i$ possible. Let $a$ be the smallest index such that $z_a$ is not among the $y_i$, then either $z_a$ is born at $t_{i+1}$ or is a combination of the $y_i$. If it is a combination of the $y_i$, then $z_a$ 
    
    Take the sequence $(z_i)$. Assume that $z_a$ is the smallest index $i$ such that $z_i \notin Z(K_{t_i})$. Then,  
    
    
    Note that the span-lengths of all cycles born at $t_{i+1}$ is determined by their death time. So let $N_1, \ldots, N_s$ be a lex.-maximal sequence death times for independent harmonic cycles generated at time $t_{i+1}$. Let $\zeta_j, j=1,\ldots,s \in \har (K_{t_{i+1}})$ be independent cycles that realize this sequence. Set $R' = R(t_i) \cup \{ \zeta_i \}$. We claim that these intervals are indeed part of the canonical barcode. %It is evident that $R'$ is a basis of $\har (K_{t_{i+1}})$. 

    To prove the claim we consider how the maximum span-length sequence of $Z(K_{t_{i+1}})$, denoted, $\rho_1 \geq \rho_2 \geq \cdots $ is constructed. Recall that we first take a cycle with maximum span-length. If this cycle is in $Z(K_{t_{i}})$ then this span length will appear as span interval with maximum length in $R(t_i) \subset R'$ by the induction hypothesis. This will be again true for the second number, etc. Let $\rho_j$ be the first appearance of a number that is not in the maximum span-length sequence for $Z(K_{t_{i}})$ (note that it can be that $\rho_j = \rho_{j-1}$, in this case $\rho_j$ is one more repetition of the same number). A realizing cycle is in $Z(K_{t_{i+1}}) - Z(K_{t_{i}})$ and it has to have the maximum span length in this set. Therefore, $\rho_j = N$ and $\zeta$ realizes $[t_{i+1},N+t_{i+1}]$. There must be $s$ of these intervals since we have $s$ independent cycles of span-length $N$ not in $K(t_i)$. Now we claim that the rest of the cycles in a sequence realizing the maximum span-length sequence for $Z(K_{t_{i+1}})$ must come from $Z(K_{t_{i}})$ and hence their span-lengths must appear among spans of $R(t_i) \subset R'$.

    To prove the claim let's assume for the sake of contradiction that a second cycle appearing in order of span-lengths $\zeta' \in Z(K_{t_{i+1}}) - Z(K_{t_{i}})$ has a span-length in the sequence, and $|span(\zeta')|\leq |span(\zeta)|$. $\zeta'$ must have a non-zero coefficient for $\sigma$ say $\beta$. Let $\alpha \neq 0$ be the coefficient of $\sigma$ in $\zeta$. We can form the cycle $\chi = \alpha/ \beta \zeta' - \zeta \in Z(K_{t_{i}})$. When $\chi$ becomes non-harmonic, i.e., at the first $t$ such that $\delta_t(\chi)\neq 0$, at least one of $\zeta'$ and $\zeta$ must also become non-harmonic. Since the death time of $\zeta$ is equal or larger than $\zeta'$, the death time of $\chi$ is at least that of $\zeta'$. Since $\chi$ already exists at time $t_{i}$ it must be that $|span(\chi)| > |span(\zeta')|$. This contradicts the selection of $\zeta'$ as it is in a space generated by cycles of larger span-length $\zeta$ and $\chi$. This finishes the argument.

    If $\sigma$ is $d+1$-dimensional, the set of $d$-cycles $Z(K_t)$ does not change and we can set $R(t_{i+1}) = R({t_i})$.

    
    
\end{proof}
\end{comment}
